# Supplementary material for: A view on coupled cluster perturbation theory using a bivariational Lagrangian formulation
Source: arXiv:1512.06552 ancillary file (2016-01-27)
Supplement: Supplementary file 1 [file si.pdf]

# Supporting information for:

# A view on coupled cluster perturbation theory using a bivariational Lagrangian formulation

Kasper Kristensen,[*,†] Janus Juul Eriksen,[*,†] Devin A. Matthews,[‡] Jeppe Olsen,[†] and Poul Jørgensen[†]

*qLEAP Center for Theoretical Chemistry, Department of Chemistry, Aarhus University, Langelandsgade 140, DK-8000 Aarhus C, Denmark, and The Institute for Computational Engineering and Sciences, The University of Texas at Austin, Austin, Texas 78712, USA*

E-mail: kasperk@chem.au.dk; janusje@chem.au.dk

[*]To whom correspondence should be addressed
[†]Aarhus University
[‡]The University of Texas at Austin

In the following, errors for the CCSDT–CCSD correlation energy difference are presented for the E-CCSD(T–$n$) series. Results are reported for mean recoveries $\Delta$ (in %) with respect to 100% and mean deviations $\delta$ (in kcal/mol) as well as standard deviations around the means ($\Delta_{\text{std}}$ and $\delta_{\text{std}}$, respectively).

In all tables, VDZ and VTZ refer to the cc-pVDZ and cc-pVTZ basis sets, respectively, and we note that the frozen-core approximation has been invoked for all the calculations reported herein.

Table S1: Recoveries of CCSDT–CCSD correlation energy differences (in %) for an RHF reference.

| Molecule | E-CCSD(T–3) | | E-CCSD(T–4) | | E-CCSD(T–5) | | E-CCSD(T–6) | | E-CCSD(T–7) | |
|---|---|---|---|---|---|---|---|---|---|---|
| | VDZ | VTZ | VDZ | VTZ | VDZ | VTZ | VDZ | VTZ | VDZ | VTZ |
| $C_2H_2$ | -9.83 | -3.01 | -12.28 | -13.65 | -2.08 | 0.33 | -2.22 | -2.58 | -1.26 | -0.75 |
| $C_2H_4$ | -18.39 | -10.56 | -12.16 | -12.19 | -4.12 | -2.07 | -2.52 | -2.27 | -1.51 | -1.14 |
| $CH_2$ ($^1A_1$) | -46.43 | -34.89 | -28.33 | -22.01 | -19.30 | -13.95 | -14.29 | -10.27 | -11.09 | -8.01 |
| $CH_2O$ | -6.50 | -1.91 | -16.55 | -15.40 | -0.23 | 1.28 | -4.18 | -3.94 | -0.38 | 0.01 |
| CO | 1.94 | 2.77 | -22.16 | -19.83 | 3.89 | 4.40 | -6.46 | -6.20 | 0.66 | 1.11 |
| $CO_2$ | 8.09 | 7.29 | -25.89 | -21.65 | 8.75 | 7.78 | -10.28 | -8.75 | 3.85 | 3.58 |
| $F_2$ | -13.66 | -4.98 | -15.98 | -14.43 | -4.55 | -1.24 | -4.03 | -3.34 | -1.70 | -0.93 |
| $H_2O$ | -11.97 | -4.30 | -7.29 | -7.79 | -1.65 | -0.37 | -0.92 | -0.88 | -0.43 | -0.42 |
| $H_2O_2$ | -11.62 | -4.10 | -11.90 | -11.68 | -2.93 | -0.59 | -2.40 | -2.14 | -1.09 | -0.70 |
| HCN | -4.33 | 0.98 | -13.61 | -15.12 | -0.79 | 1.56 | -2.60 | -3.21 | -1.01 | -0.46 |
| HF | -4.95 | -1.30 | -7.02 | -7.40 | -0.57 | 0.30 | -0.87 | -0.91 | -0.23 | -0.24 |
| HNO | -8.12 | -2.30 | -16.94 | -16.58 | -2.58 | 0.06 | -4.70 | -4.50 | -1.78 | -0.95 |
| HOF | -10.60 | -3.52 | -14.88 | -13.74 | -2.88 | -0.20 | -3.54 | -3.11 | -1.14 | -0.52 |
| $N_2$ | -1.67 | 2.97 | -13.33 | -15.04 | -0.35 | 1.98 | -2.36 | -3.08 | -0.87 | -0.37 |
| $N_2H_2$ | -11.64 | -4.74 | -13.33 | -13.82 | -3.17 | -0.75 | -2.84 | -2.87 | -1.47 | -0.99 |
| $NH_3$ | -16.31 | -8.08 | -7.61 | -8.07 | -2.18 | -0.96 | -0.94 | -0.87 | -0.51 | -0.50 |
| $O_3$ | 2.32 | 6.66 | -34.75 | -31.69 | 7.54 | 10.26 | -19.46 | -18.40 | 6.93 | 8.52 |
| $\Delta$ | -9.63 | -3.71 | -16.12 | -15.30 | -1.60 | 0.46 | -4.98 | -4.55 | -0.77 | -0.16 |
| $\Delta_{std}$ | 11.79 | 9.32 | 7.64 | 6.01 | 5.93 | 4.95 | 5.11 | 4.41 | 3.48 | 3.13 |

Table S2: Recoveries of CCSDT–CCSD correlation energy differences (in %) for a UHF reference.

| Molecule | E-CCSD(T–3) | | E-CCSD(T–4) | | E-CCSD(T–5) | | E-CCSD(T–6) | | E-CCSD(T–7) | |
|---|---|---|---|---|---|---|---|---|---|---|
| | VDZ | VTZ | VDZ | VTZ | VDZ | VTZ | VDZ | VTZ | VDZ | VTZ |
| C | -49.48 | -39.89 | -23.58 | -18.16 | -11.61 | -8.67 | -5.95 | -4.34 | -3.15 | -2.28 |
| CCH | -30.16 | -21.60 | -25.79 | -23.72 | -15.81 | -11.49 | -12.86 | -10.65 | -10.09 | -7.81 |
| CF | -3.72 | -4.51 | -26.50 | -20.33 | 3.18 | 2.09 | -10.18 | -7.60 | 1.76 | 1.26 |
| CH | -47.48 | -37.47 | -25.16 | -19.77 | -14.39 | -10.76 | -8.81 | -6.48 | -5.66 | -4.16 |
| $CH_2$ ($^3B_1$) | -34.89 | -26.42 | -14.49 | -11.94 | -6.55 | -4.95 | -3.29 | -2.45 | -1.82 | -1.37 |
| $CH_3$ | -28.48 | -19.88 | -11.88 | -10.52 | -5.02 | -3.56 | -2.46 | -1.84 | -1.41 | -1.07 |
| CN | -28.26 | -21.82 | -32.94 | -31.05 | -18.86 | -14.81 | -18.36 | -16.54 | -13.89 | -11.64 |
| F | -13.24 | -11.73 | -4.48 | -5.94 | -1.43 | -1.43 | -0.58 | -0.71 | -0.33 | -0.45 |
| HCO | -2.26 | 0.12 | -21.05 | -19.13 | 1.68 | 2.74 | -6.33 | -6.01 | 0.08 | 0.55 |
| $HO_2$ | -10.68 | -6.32 | -16.92 | -15.85 | -3.53 | -1.71 | -5.23 | -4.82 | -2.14 | -1.61 |
| N | -34.41 | -27.05 | -10.96 | -9.32 | -3.57 | -3.25 | -1.22 | -1.22 | -0.45 | -0.52 |
| NH | -32.40 | -23.55 | -13.48 | -10.63 | -6.02 | -4.13 | -3.12 | -2.05 | -1.78 | -1.14 |
| $NH_2$ | -25.13 | -16.31 | -10.74 | -9.38 | -4.41 | -2.85 | -2.23 | -1.57 | -1.28 | -0.93 |
| NO | -2.07 | 0.54 | -19.13 | -18.56 | 0.33 | 2.03 | -5.19 | -5.38 | -0.75 | -0.09 |
| O | -26.14 | -20.90 | -8.09 | -7.86 | -2.86 | -2.75 | -1.16 | -1.18 | -0.56 | -0.64 |
| $O_2$ | -2.25 | 1.05 | -13.25 | -14.38 | -0.82 | 1.15 | -2.59 | -3.01 | -0.85 | -0.43 |
| OF | -10.37 | -6.57 | -24.12 | -20.05 | -3.07 | -1.05 | -9.70 | -7.86 | -2.04 | -1.05 |
| OH | -20.72 | -13.26 | -9.51 | -8.22 | -3.52 | -2.11 | -1.92 | -1.32 | -1.06 | -0.74 |
| $\Delta$ | -22.34 | -16.42 | -17.34 | -15.27 | -5.35 | -3.64 | -5.62 | -4.72 | -2.52 | -1.89 |
| $\Delta_{std}$ | 15.07 | 12.33 | 7.78 | 6.60 | 6.07 | 4.92 | 4.75 | 4.09 | 3.81 | 3.13 |

Table S3: Recoveries of CCSDT–CCSD correlation energy differences (in %) for an ROHF reference.

| Molecule | E-CCSD(T–3) | | E-CCSD(T–4) | | E-CCSD(T–5) | | E-CCSD(T–6) | | E-CCSD(T–7) | |
|---|---|---|---|---|---|---|---|---|---|---|
| | VDZ | VTZ | VDZ | VTZ | VDZ | VTZ | VDZ | VTZ | VDZ | VTZ |
| C | -52.83 | -42.65 | -28.21 | -21.60 | -16.69 | -12.29 | -11.20 | -8.01 | -8.50 | -5.98 |
| CCH | -16.15 | -8.45 | -16.15 | -16.32 | -5.30 | -2.22 | -4.09 | -3.76 | -2.07 | -1.25 |
| CF | -3.41 | -4.37 | -26.43 | -20.33 | 3.82 | 2.54 | -9.83 | -7.37 | 2.49 | 1.79 |
| CH | -49.02 | -38.62 | -27.07 | -20.99 | -16.38 | -11.95 | -10.80 | -7.62 | -7.65 | -5.27 |
| $CH_2$ ($^3B_1$) | -35.85 | -26.99 | -15.13 | -12.17 | -6.77 | -4.88 | -3.21 | -2.17 | -1.53 | -0.96 |
| $CH_3$ | -28.75 | -20.07 | -12.00 | -10.55 | -5.00 | -3.48 | -2.33 | -1.68 | -1.21 | -0.86 |
| CN | -6.66 | -2.08 | -24.56 | -24.41 | -2.31 | 0.40 | -9.20 | -9.40 | -2.02 | -0.89 |
| F | -15.31 | -12.46 | -6.70 | -6.52 | -3.55 | -1.88 | -2.64 | -1.09 | -2.34 | -0.79 |
| HCO | -2.76 | 0.00 | -22.39 | -19.88 | 1.31 | 2.87 | -7.40 | -6.53 | -0.39 | 0.66 |
| $HO_2$ | -11.66 | -6.84 | -17.80 | -16.23 | -4.10 | -1.77 | -5.82 | -4.92 | -2.53 | -1.50 |
| N | -34.42 | -28.63 | -10.83 | -11.14 | -3.19 | -5.02 | -0.66 | -2.91 | 0.20 | -2.16 |
| NH | -34.93 | -25.01 | -16.07 | -11.87 | -8.27 | -5.09 | -5.09 | -2.81 | -3.57 | -1.77 |
| $NH_2$ | -25.93 | -16.69 | -11.38 | -9.55 | -4.84 | -2.83 | -2.51 | -1.45 | -1.45 | -0.73 |
| NO | -1.94 | 1.13 | -20.73 | -19.37 | -0.12 | 2.41 | -6.68 | -6.03 | -1.78 | -0.14 |
| O | -28.84 | -22.45 | -11.22 | -9.34 | -5.87 | -4.03 | -4.06 | -2.36 | -3.38 | -1.75 |
| $O_2$ | -13.29 | -4.41 | -23.60 | -19.41 | -12.03 | -4.07 | -13.67 | -8.19 | -11.92 | -5.50 |
| OF | -8.94 | -5.57 | -23.83 | -19.86 | -1.53 | 0.13 | -9.05 | -7.42 | -0.66 | 0.04 |
| OH | -21.92 | -13.74 | -10.65 | -8.54 | -4.48 | -2.27 | -2.77 | -1.39 | -1.83 | -0.76 |
| $\Delta$ | -21.81 | -15.44 | -18.04 | -15.45 | -5.29 | -2.97 | -6.17 | -4.73 | -2.78 | -1.55 |
| $\Delta_{std}$ | 15.50 | 13.10 | 6.72 | 5.48 | 5.40 | 4.20 | 3.73 | 2.84 | 3.40 | 2.08 |

Table S4: Deviations from CCSDT correlation energies (in kcal/mol) for an RHF reference.

| Molecule | E-CCSD(T–3) | | E-CCSD(T–4) | | E-CCSD(T–5) | | E-CCSD(T–6) | | E-CCSD(T–7) | |
|---|---|---|---|---|---|---|---|---|---|---|
| | VDZ | VTZ | VDZ | VTZ | VDZ | VTZ | VDZ | VTZ | VDZ | VTZ |
| $C_2H_2$ | 0.71 | 0.31 | 0.88 | 1.41 | 0.15 | -0.03 | 0.16 | 0.27 | 0.09 | 0.08 |
| $C_2H_4$ | 1.20 | 1.02 | 0.79 | 1.17 | 0.27 | 0.20 | 0.16 | 0.22 | 0.10 | 0.11 |
| $CH_2$ ($^1A_1$) | 1.05 | 1.23 | 0.64 | 0.78 | 0.44 | 0.49 | 0.32 | 0.36 | 0.25 | 0.28 |
| $CH_2O$ | 0.42 | 0.20 | 1.07 | 1.61 | 0.02 | -0.13 | 0.27 | 0.41 | 0.02 | 0.00 |
| CO | -0.14 | -0.30 | 1.55 | 2.12 | -0.27 | -0.47 | 0.45 | 0.66 | -0.05 | -0.12 |
| $CO_2$ | -0.92 | -1.29 | 2.95 | 3.83 | -1.00 | -1.38 | 1.17 | 1.55 | -0.44 | -0.63 |
| $F_2$ | 0.80 | 0.56 | 0.93 | 1.63 | 0.26 | 0.14 | 0.23 | 0.38 | 0.10 | 0.10 |
| $H_2O$ | 0.24 | 0.21 | 0.15 | 0.38 | 0.03 | 0.02 | 0.02 | 0.04 | 0.01 | 0.02 |
| $H_2O_2$ | 0.68 | 0.47 | 0.70 | 1.34 | 0.17 | 0.07 | 0.14 | 0.25 | 0.06 | 0.08 |
| HCN | 0.33 | -0.11 | 1.03 | 1.68 | 0.06 | -0.17 | 0.20 | 0.36 | 0.08 | 0.05 |
| HF | 0.06 | 0.05 | 0.09 | 0.30 | 0.01 | -0.01 | 0.01 | 0.04 | 0.00 | 0.01 |
| HNO | 0.62 | 0.29 | 1.30 | 2.05 | 0.20 | -0.01 | 0.36 | 0.56 | 0.14 | 0.12 |
| HOF | 0.61 | 0.40 | 0.85 | 1.55 | 0.17 | 0.02 | 0.20 | 0.35 | 0.07 | 0.06 |
| $N_2$ | 0.13 | -0.34 | 1.00 | 1.72 | 0.03 | -0.23 | 0.18 | 0.35 | 0.07 | 0.04 |
| $N_2H_2$ | 0.88 | 0.56 | 1.00 | 1.64 | 0.24 | 0.09 | 0.21 | 0.34 | 0.11 | 0.12 |
| $NH_3$ | 0.42 | 0.40 | 0.19 | 0.40 | 0.06 | 0.05 | 0.02 | 0.04 | 0.01 | 0.02 |
| $O_3$ | -0.48 | -1.91 | 7.12 | 9.11 | -1.55 | -2.95 | 3.99 | 5.29 | -1.42 | -2.45 |
| $\delta$ | 0.39 | 0.10 | 1.31 | 1.92 | -0.04 | -0.25 | 0.48 | 0.67 | -0.05 | -0.12 |
| $\delta_{\text{std}}$ | 0.54 | 0.76 | 1.63 | 2.03 | 0.50 | 0.80 | 0.94 | 1.24 | 0.38 | 0.63 |

Table S5: Deviations from CCSDT correlation energies (in kcal/mol) for a UHF reference.

| Molecule | E-CCSD(T–3) | | E-CCSD(T–4) | | E-CCSD(T–5) | | E-CCSD(T–6) | | E-CCSD(T–7) | |
|---|---|---|---|---|---|---|---|---|---|---|
| | VDZ | VTZ | VDZ | VTZ | VDZ | VTZ | VDZ | VTZ | VDZ | VTZ |
| C | 0.38 | 0.63 | 0.18 | 0.28 | 0.09 | 0.14 | 0.05 | 0.07 | 0.02 | 0.04 |
| CCH | 2.17 | 2.19 | 1.85 | 2.40 | 1.14 | 1.16 | 0.92 | 1.08 | 0.72 | 0.79 |
| CF | 0.18 | 0.38 | 1.28 | 1.73 | -0.15 | -0.18 | 0.49 | 0.65 | -0.09 | -0.11 |
| CH | 0.69 | 0.92 | 0.37 | 0.49 | 0.21 | 0.26 | 0.13 | 0.16 | 0.08 | 0.10 |
| $CH_2$ ($^3B_1$) | 0.46 | 0.64 | 0.19 | 0.29 | 0.09 | 0.12 | 0.04 | 0.06 | 0.02 | 0.03 |
| $CH_3$ | 0.59 | 0.69 | 0.25 | 0.36 | 0.10 | 0.12 | 0.05 | 0.06 | 0.03 | 0.04 |
| CN | 2.62 | 2.83 | 3.05 | 4.02 | 1.75 | 1.92 | 1.70 | 2.14 | 1.29 | 1.51 |
| F | 0.08 | 0.28 | 0.03 | 0.14 | 0.01 | 0.03 | 0.00 | 0.02 | 0.00 | 0.01 |
| HCO | 0.16 | -0.01 | 1.46 | 2.08 | -0.12 | -0.30 | 0.44 | 0.65 | -0.01 | -0.06 |
| $HO_2$ | 0.62 | 0.70 | 0.99 | 1.75 | 0.21 | 0.19 | 0.30 | 0.53 | 0.12 | 0.18 |
| N | 0.16 | 0.44 | 0.05 | 0.15 | 0.02 | 0.05 | 0.01 | 0.02 | 0.00 | 0.01 |
| NH | 0.36 | 0.62 | 0.15 | 0.28 | 0.07 | 0.11 | 0.04 | 0.05 | 0.02 | 0.03 |
| $NH_2$ | 0.46 | 0.62 | 0.20 | 0.35 | 0.08 | 0.11 | 0.04 | 0.06 | 0.02 | 0.03 |
| NO | 0.15 | -0.06 | 1.39 | 2.17 | -0.02 | -0.24 | 0.38 | 0.63 | 0.05 | 0.01 |
| O | 0.14 | 0.42 | 0.04 | 0.16 | 0.02 | 0.06 | 0.01 | 0.02 | 0.00 | 0.01 |
| $O_2$ | 0.14 | -0.12 | 0.82 | 1.60 | 0.05 | -0.13 | 0.16 | 0.33 | 0.05 | 0.05 |
| OF | 0.59 | 0.70 | 1.38 | 2.15 | 0.18 | 0.11 | 0.56 | 0.84 | 0.12 | 0.11 |
| OH | 0.25 | 0.45 | 0.11 | 0.28 | 0.04 | 0.07 | 0.02 | 0.04 | 0.01 | 0.02 |
| $\delta$ | 0.57 | 0.68 | 0.77 | 1.15 | 0.21 | 0.20 | 0.30 | 0.41 | 0.14 | 0.16 |
| $\delta_{\text{std}}$ | 0.70 | 0.73 | 0.83 | 1.12 | 0.47 | 0.53 | 0.43 | 0.55 | 0.33 | 0.39 |

Table S6: Deviations from CCSDT correlation energies (in kcal/mol) for an ROHF reference.

| Molecule | E-CCSD(T–3) | | E-CCSD(T–4) | | E-CCSD(T–5) | | E-CCSD(T–6) | | E-CCSD(T–7) | |
|---|---|---|---|---|---|---|---|---|---|---|
| | VDZ | VTZ | VDZ | VTZ | VDZ | VTZ | VDZ | VTZ | VDZ | VTZ |
| C | 0.43 | 0.70 | 0.23 | 0.35 | 0.13 | 0.20 | 0.09 | 0.13 | 0.07 | 0.10 |
| CCH | 1.16 | 0.85 | 1.16 | 1.65 | 0.38 | 0.22 | 0.29 | 0.38 | 0.15 | 0.13 |
| CF | 0.17 | 0.37 | 1.29 | 1.74 | -0.19 | -0.22 | 0.48 | 0.63 | -0.12 | -0.15 |
| CH | 0.73 | 0.97 | 0.40 | 0.53 | 0.24 | 0.30 | 0.16 | 0.19 | 0.11 | 0.13 |
| $CH_2$ ($^3B_1$) | 0.48 | 0.67 | 0.20 | 0.30 | 0.09 | 0.12 | 0.04 | 0.05 | 0.02 | 0.02 |
| $CH_3$ | 0.60 | 0.70 | 0.25 | 0.37 | 0.10 | 0.12 | 0.05 | 0.06 | 0.03 | 0.03 |
| CN | 0.62 | 0.27 | 2.27 | 3.12 | 0.21 | -0.05 | 0.85 | 1.20 | 0.19 | 0.11 |
| F | 0.09 | 0.30 | 0.04 | 0.16 | 0.02 | 0.04 | 0.02 | 0.03 | 0.01 | 0.02 |
| HCO | 0.20 | 0.00 | 1.58 | 2.19 | -0.09 | -0.32 | 0.52 | 0.72 | 0.03 | -0.07 |
| $HO_2$ | 0.69 | 0.76 | 1.05 | 1.81 | 0.24 | 0.20 | 0.34 | 0.55 | 0.15 | 0.17 |
| N | 0.16 | 0.47 | 0.05 | 0.18 | 0.02 | 0.08 | 0.00 | 0.05 | 0.00 | 0.04 |
| NH | 0.41 | 0.68 | 0.19 | 0.32 | 0.10 | 0.14 | 0.06 | 0.08 | 0.04 | 0.05 |
| $NH_2$ | 0.49 | 0.64 | 0.21 | 0.36 | 0.09 | 0.11 | 0.05 | 0.06 | 0.03 | 0.03 |
| NO | 0.14 | -0.13 | 1.55 | 2.31 | 0.01 | -0.29 | 0.50 | 0.72 | 0.13 | 0.02 |
| O | 0.16 | 0.46 | 0.06 | 0.19 | 0.03 | 0.08 | 0.02 | 0.05 | 0.02 | 0.04 |
| $O_2$ | 0.90 | 0.52 | 1.61 | 2.30 | 0.82 | 0.48 | 0.93 | 0.97 | 0.81 | 0.65 |
| OF | 0.52 | 0.60 | 1.38 | 2.14 | 0.09 | -0.01 | 0.52 | 0.80 | 0.04 | 0.00 |
| OH | 0.27 | 0.47 | 0.13 | 0.29 | 0.05 | 0.08 | 0.03 | 0.05 | 0.02 | 0.03 |
| $\delta$ | 0.46 | 0.52 | 0.76 | 1.13 | 0.13 | 0.07 | 0.28 | 0.37 | 0.10 | 0.07 |
| $\delta_{\text{std}}$ | 0.29 | 0.28 | 0.72 | 1.00 | 0.21 | 0.20 | 0.30 | 0.38 | 0.19 | 0.16 |
